# Supplementary material for: Neural Graph Embedding Methods for Natural Language Processing
Source: arXiv:1911.03042 source file (2020-04-07)
Supplement: Supplementary file 1 [file appendix.tex]

\subsection{Evaluation by Relation Category}
\label{compgcn_sec:results_rel_cat}
In this section, we investigate the performance of \textsc{CompGCN} on link prediction for different relation categories on FB15k-237 dataset. Following \citet{kg_relation_cat,rotate}, based on the average number of tails per head and heads per tail, we divide the relations into four categories: one-to-one, one-to-many, many-to-one and many-to-many. The results are summarized in Table \ref{compgcn_tbl:results_rel_cat}. We observe that using GCN based encoders for obtaining entity and relation embeddings helps to improve performance on all types of relations. In the case of one-to-one relations, \textsc{CompGCN} gives an average improvement of around $10$\% on MRR compared to the best performing baseline (ConvE + W-GCN). For one-to-many, many-to-one, and many-to-many the corresponding improvements are $10.5$\%, $7.5$\%, and $4$\%. These results show that \textsc{CompGCN} is effective at handling both simple and complex relations.

\begin{table*}[!h]
	\centering
	\small
	\begin{tabular}{lm{3em}ccccccccccc}
		\toprule
		
		{} &  {} & \multicolumn{3}{c}{\textbf{ConvE}} && \multicolumn{3}{c}{\textbf{ConvE + W-GCN}} && \multicolumn{3}{c}{\textbf{ConvE + \textsc{CompGCN} (Corr)}} \\
		\cmidrule(r){3-5}  \cmidrule(r){7-9} \cmidrule(r){11-13}
		{} & &   MRR & MR   & H@10  &&  MRR & MR   & H@10  &&  MRR & MR   & H@10   \\
		\midrule
		\multirow{4}{*}{\rotatebox[origin=c]{90}{Head Pred}} & 1-1 & 0.193	& 459	& 0.385	&& 0.422	& 238	& 0.547	&& \textbf{0.457	}& \textbf{150}	& \textbf{0.604} \\
		& 1-N & 0.068	& 922	& 0.116	&& 0.093	& 612	& 0.187	&& \textbf{0.112}	& \textbf{604}	& \textbf{0.190} \\
		& N-1 & 0.438	& 123	& 0.638	&& 0.454	& 101	& 0.647	&& \textbf{0.471}	& \textbf{99}	& \textbf{0.656} \\
		& N-N & 0.246	& 189	& 0.436	&& 0.261	& \textbf{169}	& 0.459	&& \textbf{0.275} & 179	& \textbf{0.474} \\
		\midrule
		\multirow{4}{*}{\rotatebox[origin=c]{90}{Tail Pred}} & 1-1 & 0.177	& 402	& 0.391	&& 0.406	& 319	& 0.531	&& \textbf{0.453}	& \textbf{193}	& \textbf{0.589} \\
		& 1-N & 0.756	& 66	& 0.867	&& 0.771	& 43	& 0.875	&& \textbf{0.779}	& \textbf{34}	& \textbf{0.885} \\
		& N-1 & 0.049	& 783	& 0.09	&& 0.068	& \textbf{747}	& 0.139	&& \textbf{0.076}	& 792	& \textbf{0.151} \\
		& N-N & 0.369	& 119	& 0.587	&& 0.385	& 107	& 0.607	&& \textbf{0.395	}& \textbf{102}	& \textbf{0.616} \\
		\bottomrule
	\end{tabular}
	\caption{\label{compgcn_tbl:results_rel_cat}Results on link prediction by relation category on FB15k-237 dataset. Following \cite{kg_relation_cat}, the relations are divided into four categories: one-to-one (1-1), one-to-many (1-N), many-to-one (N-1), and many-to-many (N-N). We find that \textsc{CompGCN} helps to improve performance on all types of relations compared to existing methods. Please refer to Section \ref{compgcn_sec:results_rel_cat} for more details.}
\end{table*}

\subsection{Dataset Statistics}
\label{compgcn_sec:dataset_stats}

In Table \ref{compgcn_table:rgcn_data}, we provide the statistics of the datasets used for link prediction, node classfication, and graph classification tasks. 
\begin{table}[h]
	\centering
	\small
	\begin{tabular}{lcccccc}
		\toprule
		&  \multicolumn{2}{c}{\bf Link Prediction} & \multicolumn{2}{c}{\bf Node Classification} & \multicolumn{2}{c}{\bf Graph Classification}\\ 
		\cmidrule(r){2-3} \cmidrule(r){4-5} \cmidrule(r){6-7} 
		& \multicolumn{1}{c}{FB15k-237} & \multicolumn{1}{c}{WN18RR} & \multicolumn{1}{c}{MUTAG (Node)} &  \multicolumn{1}{c}{AM} & \multicolumn{1}{c}{MUTAG (Graph)} & \multicolumn{1}{c}{PTC}\\
		\midrule
		Graphs   & 1 & 1 & 1 & 1 & 188 & 344 \\
		Entities   & 14,541 & 40,943 & 23,644 & 1,666,764 & 17.9 (Avg) & 25.5 (Avg)\\
		Edges 	  & 310,116 & 93,003 & 74,227 & 5,988,321 & 39.6 (Avg) & 29.5 (Avg)\\
		Relations & 237 & 11 & 23 & 133 & 4 & 4 \\
		%		Labeled   & - & - & 340 & 1000 & - & -\\
		Classes   & - & - & 2 & 11 & 2 & 2\\
		\bottomrule
	\end{tabular}
	
	\caption{\label{compgcn_table:rgcn_data}The details of the datasets used for node classification, link prediction, and graph classification tasks. Please refer to Section \ref{compgcn_sec:exp_tasks} for more details.}
\end{table}

\subsection{Hyperparameters}
\label{compgcn_sec:hyperparams}
Here, we present the implementation details for each task used for evaluation in the chapter. For all the tasks, we used \textsc{CompGCN} build on PyTorch geometric framework \citep{pytorch_geometric}. 

\noindent \textbf{Link Prediction:} For evaluation, $200$-dimensional embeddings for node and relation embeddings. For selecting the best model we perform a hyperparameter search using the validation data over the values listed in Table \ref{compgcn_table:hyperparams}. 

\noindent \textbf{Node Classification:} Following \citet{r_gcn}, we use $0.1$\% training data as validation for selecting the best model for both the datasets. We restrict the number of hidden units to $32$. %and GCN layers to $2$. 

\noindent \textbf{Graph Classification:} Similar to \cite{graph_datasets,gin}, we report the average and standard deviation of validation accuracies across the 10 folds cross-validation.
%\noindent \textbf{Neural Machine Translation:} We utilize OpenNMT \cite{opennmt} as our building framework.  For Multi30k, we keep hidden units to 256 while for News commentary dataset we use 512 hidden units. Similar to \citet{gcn_mt}. for all the models, we restrict to $1$-layer of GCN. For $L2$, we search in the range $[0.0001, 0.00001]$ and for dropout we search over $\{0.2, 0.3, 0.4, 0.5\}$ using the provided validation data. 

For all the experiments, training is done using Adam optimizer \citep{adam_opt} and Xavier initialization \citep{xavier_init} is used for initializing parameters.
	
\begin{table}[h]
	\centering
	\small
	\begin{tabular}{ll}
		\toprule
		Hyperparameter                 & Values 					\\
		\midrule
		Number of GCN Layer ($K$) & \{1, 2, 3\}			\\
		Learning rate                  & \{0.001, 0.0001\}			\\
		Batch size                     & \{128, 256\}			\\
		Dropout  & \{0.0, 0.1, 0.2, 0.3\}		\\
		\bottomrule
	\end{tabular}
	\caption{Details of hyperparameters used for link prediction task. Please refer to Section \ref{compgcn_sec:hyperparams} for more details.}
	\label{compgcn_table:hyperparams}
\end{table}
